# Supplementary material for: Construction Sequences and Certifying 3-Connectedness
Source: arXiv:0912.2561 source file (2010-02-03)
Supplement: Supplementary file 1 [file Appendix.tex]

\begin{lemma}[4.1]
The edge and path representations of a construction sequence $Q$ can be transformed into each other in $O(m)$. Moreover, the representation computed is a unique representation of $Q$.
\end{lemma}
\begin{proof}
Let $G_0$ and a sequence of \BG-operations along with their specified indices on edges and nodes be given. If an operation $O'$ subdivides an edge $e'$, we define $\beta(e',O')$ to be the edge of the two new ones that gets a new index. Let $e$ be the added edge of an operation in $Q$. With the preliminary considerations $e$ corresponds to a \BG-path $C$ and will therefore be subdivided $|C|-1$ times in the construction sequence. To compute the \BG-path $C$ we have to keep track of the $|C|-1$ operations that subdivide $e$ and glue the subdivided parts back together.

Whenever an operation $O \in Q$ subdivides $e$ we store a pointer to $e$ at $\beta(e,O)$. Moreover, on all edges $f$ that are subdivided and point to $e$ we store a pointer to $e$ at $\beta(f,O'')$. In both cases, we append $\beta(e,O)$ resp. $\beta(f,O'')$ to a list stored on the edge $e$. Each $\beta(e,O)$ and $\beta(f,O'')$ can be found in constant time and by augmenting the list of $e$ with $e$ itself we get all the edges in which $C$ got subdivided in the end, hence exactly the set of edges in the \BG-path $C$. Since $G_z$ has the same labeling as $G$, the indices of $e$ and all other edges in $C$ are still contained in $G$.

The set of edges is not necessarily in the order of appearance in $C$, but this can be easily fixed in time $O(|C|)$ by temporarily storing the incidence information of every node in $C$ and extracting the \BG-path $C$ from a degree-one node. In order to compute $S_0$, we analogously maintain pointers for each edge of $G_0$ and get the links of $S_0$. Since the links of $S_0$ together with $C_0,\ldots,C_{z-1}$ partition $E(G) \setminus E(S_0)$, the running time is $O(m)$.

Conversely, let $S_0$ and the sequence $C_0,\ldots,C_{z-1}$ of \BG-paths be given. We \emph{remove} \BG-paths in reversed order from $G$ by deleting their edge (there is only one edge left this way, the one added in the corresponding \BG-operation) followed by smoothing their endnodes. Therefore, we pass through the graph sequence $G_z,\ldots,G_0$ and get $G_0$. If both endnodes of the \BG-path $C_i=a \rightarrow b$ are real after deleting $ab$, we can keep their index and construct the corresponding \BG-operation~\ref{operation1}.

Otherwise, let $a$ have degree $2$ after deleting $ab$ and let $e$ and $f$ be its incident edges. When $a$ is smoothed we can assign the lowest index of $e$ and $f$ to the new edge, thus, all indices that are necessary for constructing the operation~\ref{operation2} can be found in constant time. If additionally $b$ has degree $2$, the same procedure constructs operation~\ref{operation3}. It remains to show that always unique representations of $Q$ are computed. The path representation with \BG-paths is by definition unique. Edge representations can vary in their indices, but picking the incident edge with lowest index before smoothing a node creates a unique representation, since all edge indices of $G$ are given.
\end{proof}

\begin{lemma}[5.1]
For simple graphs $G$, the construction sequences~\eqref{theoremitem1} and~\eqref{theoremitem2} can be transformed into each other in $O(m)$.
\end{lemma}
\begin{proof}
Let the construction sequence~\eqref{theoremitem1} in the path representation be given. For each \BG-path $P$, its position in the construction sequence and a pointer to the first \BG-path $F(P)$ that ends at an inner node of $P$ (if that path exists) is stored. We define the position of each link of $S_0$ as $0$. Performing a bucket sort on the endnodes of \BG-paths with lower id followed by a stable bucket sort on the remaining endnodes gives a list of paths sorted in lexicographic order of the endnode ids. This list can be used to efficiently group paths that have the same endnodes.

Let $S_{ab}$ be the set of all \BG-paths and links of $S_0$ having endnodes $a$ and $b$. We apply the following procedure: If a path $P \in S_{ab}$ has length one and does not have the first position of all paths in $S_{ab}$, we append it to the end of the construction sequence and remove it from $S_{ab}$. This does not harm the construction sequence, since $a$ and $b$ were already real and $P$ has no inner nodes.

The path with the first position in $S_{ab}$ cannot lead to a non-basic operation. We look at all other paths $P \in S_{ab}$, which are possibly non-basic, but must contain an inner node $w$ that is endnode of the subsequent \BG-path $F(P) = v~\rightarrow~w$. Without harming the construction sequence, $P$ can be moved to the position of $F(P)$, since $a$ and $b$ were already real and no inner node of $P$ is part of a \BG-path before $F(P)$ is applied. If $v$ is real at the point in time when $F(P)$ is applied, we can glue $P$ and $F(P)$ together to an expand operation, which is basic due to its new node $w$. Otherwise, $v$ is an inner node of a link (see Figure~\ref{fig:notexpand}) and $P$ and $F(P)$ can be replaced with the two \BG-paths $v \rightarrow a$ and $bw$. Both \BG-paths are basic, since they contain endnodes of degree $2$.

Conversely, the three internally node-disjoint paths of each expand operation can be easily split into two \BG-paths, possibly inducing non-basic operations.
\end{proof}
